# Supplementary material for: How well do we know the neutron-matter equation of state at the densities inside neutron stars? A Bayesian approach with correlated uncertainties
Source: arXiv:2004.07232 ancillary file (2021-01-07)
Supplement: Supplementary file 1 [file Supp_Mat.pdf]

# Supplemental material for "How well do we know the neutron-matter equation of state at the densities inside neutron stars? A Bayesian approach with correlated uncertainties"

C. Drischler,[1,2,*] R. J. Furnstahl,[3,†] J. A. Melendez,[3,‡] and D. R. Phillips[4,§]

[1] *Department of Physics, University of California, Berkeley, California 94720, USA*
[2] *Nuclear Science Division, Lawrence Berkeley National Laboratory, Berkeley, California 94720, USA*
[3] *Department of Physics, The Ohio State University, Columbus, Ohio 43210, USA*
[4] *Department of Physics and Astronomy and Institute of Nuclear and Particle Physics, Ohio University, Athens, Ohio 45701, USA*

(Dated: January 7, 2021)

## ADDITIONAL FIGURES

In parallel to the results shown in the main text, we provide here the corresponding figures obtained using the $\Lambda = 450\,\mathrm{MeV}$ potentials of Ref. [1] with $c_D = 2.25$ (0.00) and $c_E = 0.07$ ($-1.32$) at $\mathrm{N^2LO}$ ($\mathrm{N^3LO}$). More details—including our model-checking diagnostics for these potentials—can be found in our companion paper [2].

Figure 1 shows our order-by-order $\chi$EFT predictions, up to $\mathrm{N^3LO}$, for $\frac{E}{N}(n)$, $P(n)$, and $c_s^2(n)$ in pure neutron matter as well as $S_2(n)$, $L(n)$, and $\frac{E}{A}(n)$.

Figure 2 depicts constraints in the $S_v$–$L$ plane, with our result again represented by the yellow ellipse. Its centroid is slightly shifted toward larger $S_v$ and $L$ values compared to the results for the $\Lambda = 500\,\mathrm{MeV}$ potentials. But the $2\sigma$ ellipse still has good overlap with the region derived from multiple experimental constraints, and falls completely within the bounds derived from the conjecture that the unitary gas is a lower limit on the EOS [3] (solid black line). At $\mathrm{N^2LO}$ and $\mathrm{N^3LO}$, respectively, the distribution is accurately approximated by a two-dimensional Gaussian with mean and covariance

$$\begin{bmatrix}\mu_{S_v}\\ \mu_L\end{bmatrix} = \begin{bmatrix}34.7\\ 60.8\end{bmatrix} \quad\text{and}\quad \Sigma = \begin{bmatrix}2.32^2 & -0.44\\ -0.44 & 7.64^2\end{bmatrix}, \qquad (1)$$

$$\begin{bmatrix}\mu_{S_v}\\ \mu_L\end{bmatrix} = \begin{bmatrix}33.5\\ 67.8\end{bmatrix} \quad\text{and}\quad \Sigma = \begin{bmatrix}1.25^2 & 3.06\\ 3.06 & 4.00^2\end{bmatrix}. \qquad (2)$$

Note that we self-consistently use $n_0 = 0.17 \pm 0.02\,\mathrm{fm^{-3}}$ ($n_0 = 0.17 \pm 0.01\,\mathrm{fm^{-3}}$) at $\mathrm{N^2LO}$ ($\mathrm{N^3LO}$). For more details on the nuclear saturation point, see Section III.C in the companion paper [2].

For completeness, we also give the mean and variance of the $\mathrm{N^2LO}$ results corresponding to Figure 2 in the main text [for $\mathrm{N^3LO}$ see Eq. (5)],

$$\begin{bmatrix}\mu_{S_v}\\ \mu_L\end{bmatrix} = \begin{bmatrix}32.5\\ 60.3\end{bmatrix} \quad\text{and}\quad \Sigma = \begin{bmatrix}2.24^2 & 4.92\\ 4.92 & 6.88^2\end{bmatrix}. \qquad (3)$$

As stated in the main text, our set of $\chi$EFT NN and 3N Hamiltonians leads to $L$ values that are $\approx 10\,\mathrm{MeV}$ higher than those from two other theoretical calculations compiled by Lattimer *et al.* (see discussion of Figure 2).

Our range [$L = 59.8 \pm 4.1\,\mathrm{MeV}$] significantly overlaps with the $\mathrm{N^3LO}$ neutron matter calculations in Ref. [4], $L = 43.0 - 66.6\,\mathrm{MeV}$. Our EFT truncation-error analysis also agrees with the simple estimate in Ref. [1] (see Figure 5). Furthermore, the Quantum Monte Carlo calculations in Ref. [5] predict $P(n_0) = 2.4 \pm 0.6\,\mathrm{MeV\,fm^{-3}}$ for the local potential $V_{E,1}$ (see Table 2 in that paper). Within the uncertainties this is consistent with our result from nonlocal $\mathrm{N^2LO}$ potentials, $P(n_0) \approx 2.9 \pm 0.4\,\mathrm{MeV\,fm^{-3}}$. Since $P(n_0) \simeq n_0 \frac{L}{3}$, we can assume the estimated ranges in $L$ are consistent as well.

Notice that the (relatively large) uncertainties in $n_0$ also contribute to the uncertainties we quote for $P(n_0)$, $L(n_0)$, etc. In the literature the uncertainty in the evaluation point is often not accounted for, instead the dependent variable and its uncertainty are just evaluated at a fixed point, e.g., $n_0 = 0.16\,\mathrm{fm^{-3}}$.

Valid EFTs with the same physics content should yield the same predictions within uncertainties (independent of the fit protocol, regularization scheme, etc.)—if all uncertainties are properly accounted for. This validation among different EFT implementations has not been possible yet. In practice, the actual implementation of $\chi$EFT interactions can lead to (somewhat) different predictions. For example, while this work already accounts for correlated EFT truncation errors in the observables, the low-energy couplings in the underlying nuclear interactions are still treated as perfectly known.

A full Bayesian analysis via Markov Chain Monte Carlo sampling over GP hyperparameters and the low-energy couplings would provide a complete accounting regarding the different choices of input data and missing truncation errors for the parameter estimation. Work along these lines is progress; see, e.g., Ref. [6]. Further investigation of the underlying nuclear interactions and, in particular, the development of other order-by-order $\chi$EFT NN and 3N potentials up to $\mathrm{N^3LO}$ is also needed. The various choices regarding these potentials that need to be considered include the $\chi$EFT order (or orders, if NN and many-body forces are treated differently), fit protocol, regulator scheme, and resolution scale; each contributes to the observations in a nontrivial way.

Finally, we point out again that the correlations between the order-by-order contributions to the PNM and SNM EOS yield more accurate constraints on the symmetry energy (as the *difference* between the PNM and SNM EOS) than are obtained for each EOS individually (see also the companion paper [2]). This bears on the question of how far the physics in $\chi$EFT that shifts the energy of SNM at saturation to the empirical range will affect our results. Mechanisms in next-generation order-by-order $\chi$EFT interactions could shift the SNM EOS towards the empirical saturation point. Even then, our constraints on $S_v$ will only change significantly if those mechanisms generate *uncorrelated* (or anti-correlated) changes in the PNM EOS.

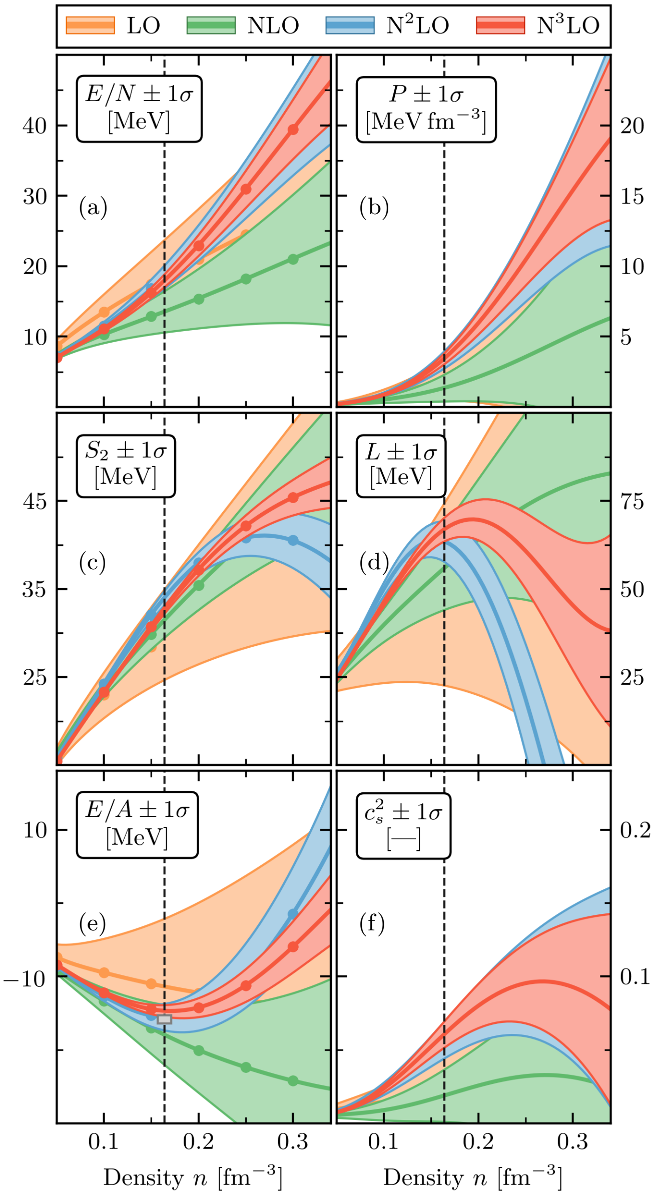


FIG. 1. The analog of Fig. 1 in the main text, but for the $\Lambda = 450$ MeV NN potentials (and corresponding 3N interactions) of Refs. [1, 7]. Order-by-order predictions with 68% bands for (a) the energy per particle $\frac{E}{N}(n)$ and (b) the pressure $P(n)$ of PNM; (c) the symmetry energy $S_2(n)$ and (d) its (rescaled) density dependence $L(n)$; (e) the energy per particle $\frac{E}{A}(n)$ of SNM; and (f) the speed of sound $c_s^2(n)$ of PNM, each as a function of density. Dots denote every fifth interpolation point, where $n = 0.05, 0.06, \ldots, 0.34\,\mathrm{fm}^{-3}$. The grey box in (e) depicts the empirical saturation point, $n_0 = 0.164 \pm 0.007\,\mathrm{fm}^{-3}$ with $\frac{E}{A}(n_0) = -15.86 \pm 0.57$ MeV, obtained from a set of energy density functionals [1, 8]. The vertical lines are located at $n = 0.164\,\mathrm{fm}^{-3}$. See the main text for details.


* cdrischler@berkeley.edu
† furnstahl.1@osu.edu
‡ melendez.27@osu.edu
§ phillid1@ohio.edu



[1] C. Drischler, K. Hebeler, and A. Schwenk, Phys. Rev. Lett. **122**, 042501 (2019), arXiv:1710.08220.
[2] C. Drischler, J. A. Melendez, R. J. Furnstahl, and D. R. Phillips, Phys. Rev. C **102**, 054315 (2020), companion paper, arXiv:2004.07805.
[3] I. Tews, J. M. Lattimer, A. Ohnishi, and E. E. Kolomeitsev, Astrophys. J. **848**, 105 (2017), arXiv:1611.07133.
[4] I. Tews, T. Krüger, K. Hebeler, and A. Schwenk, Phys. Rev. Lett. **110**, 032504 (2013), arXiv:1206.0025.
[5] I. Tews, J. Carlson, S. Gandolfi, and S. Reddy, Astrophys. J. **860**, 149 (2018), arXiv:1801.01923.
[6] S. Wesolowski, R. J. Furnstahl, J. A. Melendez, and D. R. Phillips, J. Phys. G **46**, 045102 (2019), arXiv:1808.08211.
[7] D. R. Entem, R. Machleidt, and Y. Nosyk, Phys. Rev. C **96**, 024004 (2017), arXiv:1703.05454.
[8] C. Drischler, K. Hebeler, and A. Schwenk, Phys. Rev. C **93**, 054314 (2016), arXiv:1510.06728.
[9] M. B. Tsang, Y. Zhang, P. Danielewicz, M. Famiano, Z. Li, W. G. Lynch, and A. W. Steiner, Phys. Rev. Lett. **102**, 122701 (2009), arXiv:0811.3107.
[10] L.-W. Chen, C. M. Ko, B.-A. Li, and J. Xu, Phys. Rev. C **82**, 024321 (2010), arXiv:1004.4672.
[11] L. Trippa, G. Colo, and E. Vigezzi, Phys. Rev. C **77**, 061304(R) (2008), arXiv:0802.3658.
[12] A. Tamii, I. Poltoratska, P. von Neumann-Cosel, Y. Fujita, T. Adachi, *et al.*, Phys. Rev. Lett. **107**, 062502 (2011), arXiv:1104.5431.
[13] X. Roca-Maza, M. Brenna, G. Colò, M. Centelles, X. Viñas, B. K. Agrawal, N. Paar, D. Vretenar, and J. Piekarewicz, Phys. Rev. C **88**, 024316 (2013), arXiv:1307.4806.
[14] T. Kortelainen, M. Lesinski, J. Moré, W. Nazarewicz, J. Sarich, N. Schunck, M. V. Stoitsov, and S. Wild, Phys. Rev. C **82**, 024313 (2010), arXiv:1005.5145.
[15] P. Danielewicz, P. Singh, and J. Lee, Nucl. Phys. A **958**, 147 (2017), arXiv:1611.01871.
[16] K. Hebeler, J. M. Lattimer, C. J. Pethick, and A. Schwenk, Phys. Rev. Lett. **105**, 161102 (2010), arXiv:1007.1746.
[17] S. Gandolfi, J. Carlson, and S. Reddy, Phys. Rev. C **85**, 032801(R) (2012), arXiv:1101.1921.
[18] J. M. Lattimer and A. W. Steiner, Eur. Phys. J. A **50**, 40 (2014), arXiv:1403.1186.

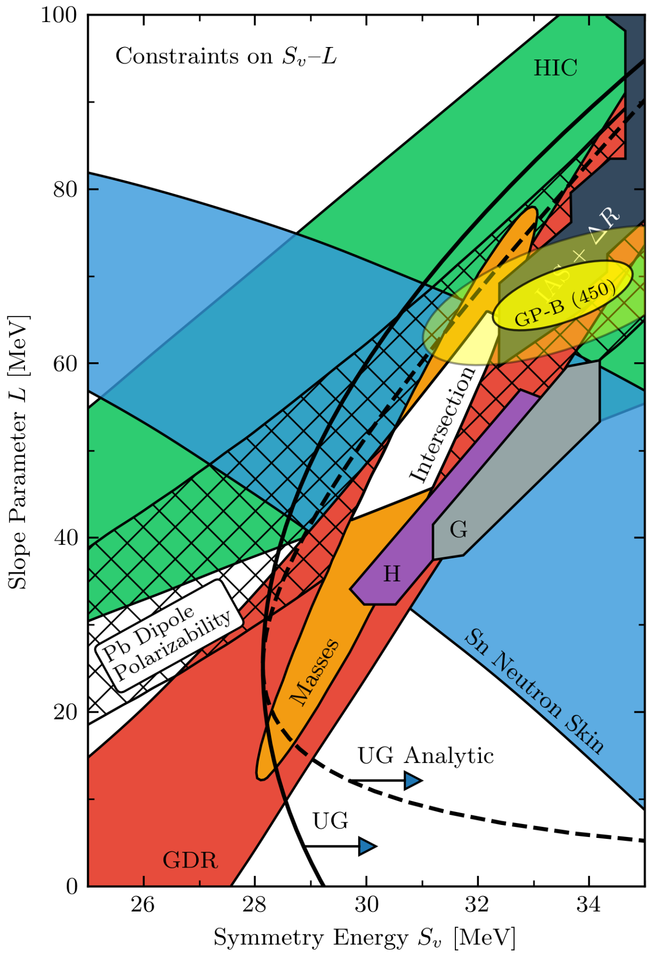


FIG. 2. The same as Fig. 2 in the main text, but with our results ("GP–B (450)") derived using the $\Lambda = 450$ MeV NN potential (and corresponding 3N interactions) of Refs. [1, 7]. Constraints on the $S_v$–$L$ correlation. Our results are given at the 68% (dark-yellow ellipse) and 95% level (light-yellow ellipse). Experimental constraints are derived from heavy-ion collisions (HIC) [9], neutron-skin thicknesses of Sn isotopes [10], giant dipole resonances (GDR) [11], the dipole polarizability of $^{208}$Pb [12, 13], and nuclear masses [14]. The intersection is depicted by the white area, which only barely overlaps with constraints from isobaric analog states and isovector skins (IAS + $\Delta R$) [15]. In addition, theoretical constraints derived from microscopic neutron-matter calculations by Hebeler *et al.* (H) [16] and Gandolfi *et al.* (G) [17] as well as from the unitary gas (UG) limit by Tews *et al.* [3]. The figure has been adapted from Refs. [18, 19]. A Jupyter notebook that generates the figure is provided in Ref. [20].


[19] J. M. Lattimer and Y. Lim, Astrophys. J. **771**, 51 (2013), arXiv:1203.4286.

[20] BUQEYE collaboration, `https://buqeye.github.io/software/`.
